# Supplementary material for: A Non-Equilibrium Dissipation Parameter and the Ideal Glass
Source: arXiv:2509.23266 source file (2025-09-27)
Supplement: Supplementary file 1 [file Supplementary_Material.pdf]

# Supplementary Material for “A Non-Equilibrium Dissipation Parameter and the Ideal Glass”

Jun-Ying Jiang<sup>1,\*</sup>, Liang Gao<sup>1,\*</sup> and Hai-Bin Yu<sup>1,†</sup>

<sup>1</sup>Wuhan National High Magnetic Field Center and School of Physic,  
Huazhong University of Science and Technology, Wuhan 430074, Hubei, China

(Dated: July 9, 2025)

This Supplementary Material provides detailed descriptions of the glass model preparation, dynamic mechanical simulations, and IS  $D_{\min}$  algorithms. Additionally, the data analysis section outlines the process of determining  $T_0$  using the Vogel-Fulcher Tamman equations and dynamic data under various simulation strategies.

## Molecular dynamics simulations and DMS

An open-source molecular dynamics simulation code, LAMMPS [1, 2], is used for all the simulations. The  $\text{Ni}_{65}\text{Nb}_{35}$  [3] and 80:20 Kob-Andersen [4] models contain 9088 and 70304 atoms, respectively. The  $\text{Ni}_{80}\text{P}_{20}$ ,  $\text{Cu}_{50}\text{Zr}_{50}$  and  $\text{Al}_{90}\text{Sm}_{10}$  models (the data for these models come from [5]) contain 32000 atoms. The preparation of These glass models are initiated using the melt-quench method that involves the following two steps: the first step is to anneal at a high temperature above the melting point until its energy stabilizes, thereby producing a high-temperature equilibrium liquid. The second step is to cool this liquid to below room temperature (the final temperature of the Kob-Andersen mixtures is below 0.2, shown in Fig.S1).

The time step is set to 1 fs during the annealing process and 2 fs during cooling (0.001 and 0.002 for the Kob-Andersen model, respectively). In these two processes, periodic boundary conditions and a Nosé-Hoover thermostat are applied in all simulations. Additionally, the  $\text{Ni}_{65}\text{Nb}_{35}$ ,  $\text{Ni}_{80}\text{P}_{20}$ ,  $\text{Cu}_{50}\text{Zr}_{50}$  and  $\text{Al}_{90}\text{Sm}_{10}$  models are simulated in an NPT ensemble, while the Kob-Andersen model is simulated in an NVT ensemble with a density of 1.2.

The Molecular Dynamics simulations of Dynamic Mechanical Spectra (MD-DMS) are designed to numerically mimic the protocol of real Dynamic Mechanical Analysis. Specifically, a sinusoidal volume-preserving strain  $\varepsilon(t) = \varepsilon_0 \sin(\omega t)$  is applied at selected time interval, with strain amplitude  $\varepsilon$  along the  $x$ - $y$  direction of the simulation box. The resulting shear stress  $\sigma$  is fitted by  $\sigma(t) = \sigma_0 \sin(\omega t + \delta)$ . From this, the storage ( $G'$ ) and loss shear modulus ( $G''$ ) are calculated from

$$G' = \frac{\sigma_0}{\varepsilon_0} \cos \delta, G'' = \frac{\sigma_0}{\varepsilon_0} \sin \delta.$$

A strain amplitude  $\gamma_A = 1.2\%$  is applied in all the MD-DMS simulations for the Kob-Andersen model. The strain amplitudes applied by the  $\text{Ni}_{65}\text{Nb}_{35}$ ,  $\text{Ni}_{80}\text{P}_{20}$ ,  $\text{Cu}_{50}\text{Zr}_{50}$ ,  $\text{Al}_{90}\text{Sm}_{10}$  models are: 2.0%, 1.4%, 1.2%, 0.7%. Such a value of strain amplitude ensures the deformation is in the linear response regime.

We determine the  $\alpha$  relaxation time  $\tau_\alpha$  and the characteristic period  $t_w$  from the peak time of the isothermal and equilibrium MD-DMS. Afterwards, these data can be well fitted by a Vogel-Fulcher-Tammann (VFT) function [6, 7],  $\tau_\alpha = \tau_0 \exp(DT_0/(T - T_0))$ , to obtain the ideal glass transition temperature  $T_0$ .

## Computation details for IS $D_{\min}$

The inherent structures (IS) are used in this work for the calculation of IS  $D_{\min}$ . They are obtained by performing an energy minimization of the system, by iteratively adjusting atom coordinates. At that point, the configuration will be at a local minimum on the potential energy surface and the influence from atomic vibrations will be removed. Specifically, we used the conjugate gradient (CG) algorithm as implemented in LAMMPS for the calculations.

First, for two consecutive ISs, the  $N \times N$  cost (displacement,  $r$ ) matrix for atom pairs  $i$  and  $j$  is defined by Eq. 1:

---

\* These authors contributed equally.

† haibinyu@hust.edu.cn

$$C_{i,j}(t) = |r_i(t + t_0) - r_j(t_0)| \quad (1)$$

Define  $X$  as an  $N \times N$  Boolean matrix, where  $X[i, j] = 1$  if the row  $i$  is assigned to the column  $j$ , and 0 otherwise. The IS  $D_{\min}$  is obtained by optimizing  $X$  to minimize the sum of the product of  $C$  and  $X$ , as shown in Eq.2:

$$\text{IS } D_{\min}(t) = \left[ \frac{1}{N} \min \sum_{i,j}^{N,N} C_{ij}(t) X_{ij}(t) \right]^{1/2} \quad (2)$$

In implementing the calculation of Eq. (1), we used the `linear_sum_assignment` function[8] from the `scipy` package for Python . It takes the cost matrix  $C_{i,j}$  as one of the input parameters and returns the optimum assignments that minimize the sum of the product of  $C$  and  $X$  in Equation (1) (i.e., one does not need to construct  $X$  by hand, more details can be found in the code).

Obviously, if the optimum  $X$  is the unit matrix, then Equation (1) is reduced to the common RMSD. This condition occurs when all atoms have small displacements ( $\Delta r_i \ll r_0/2$ ). We note that the memory cost for the computation of IS  $D_{\min}$  is at the order  $O(N^2)$ .

### Data analysis

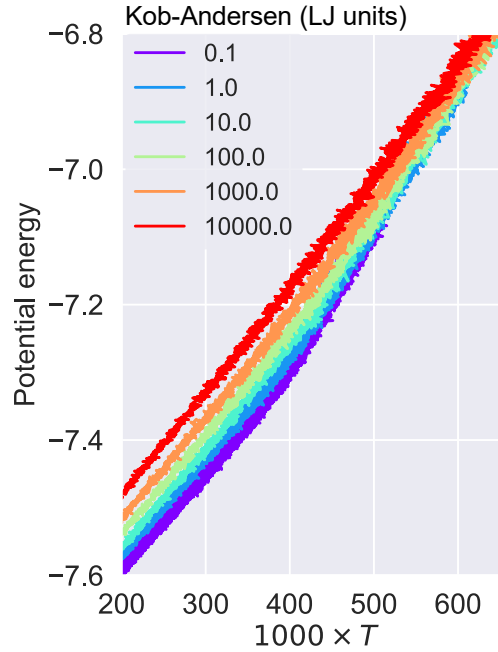

FIG. S1. Potential energy as a function of temperature for Kob-Andersen model (LJ units) under 6 different cooling rates. The model liquids at each temperature are equilibrated.

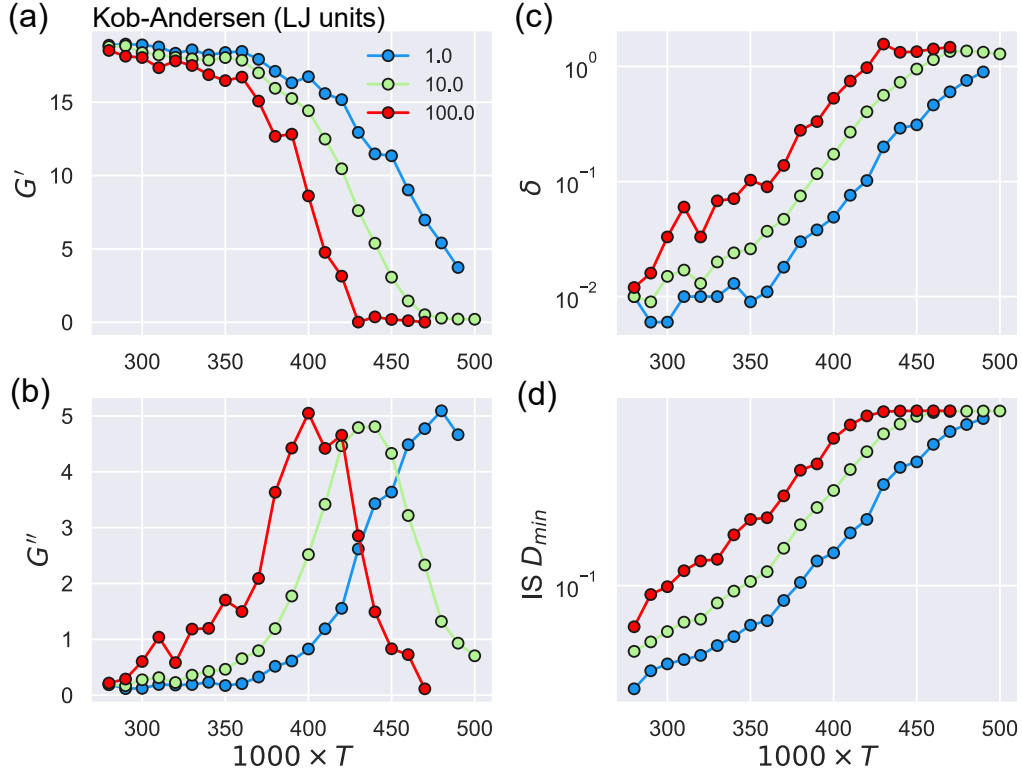

FIG. S2. Relaxation dynamics of the Kob-Andersen model (LJ units) by different  $t_\omega$  MD-DMS under the slowest cooling. (a) Storage shear modulus  $G'$ , (b) loss shear modulus  $G''$ , (c) phase angle  $\delta$  and (d) IS  $D_{min}$ .

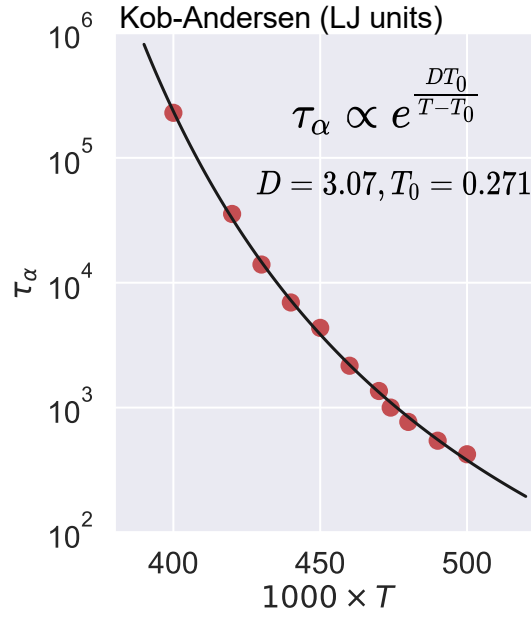

FIG. S3. The curve is fitted using the Vogel-Fulcher Tamman (VFT) equation  $\tau_\alpha = \tau_0 \exp(DT_0/T - T_0)$ , based on the peak times from isothermal and equilibrium MD-DMS measurements. The  $\alpha$ -relaxation time is determined to follow:  $\tau_\alpha \propto \exp(DT_0/T - T_0)$ , where the fragility parameter  $D = 3.07$  and the divergence temperature  $T_0 = 0.27$ .

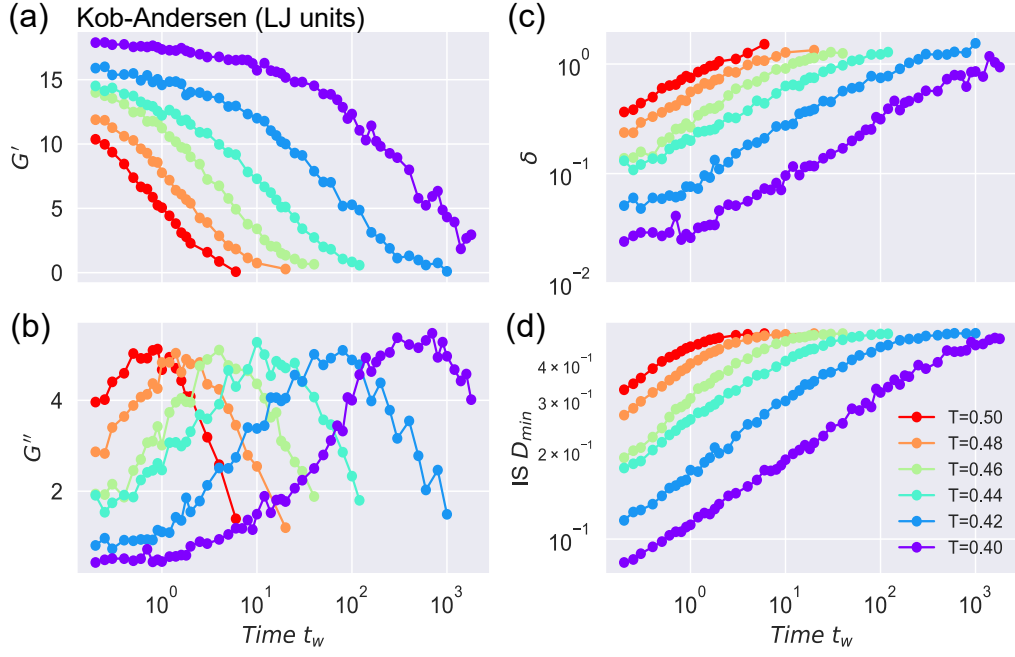

FIG. S4. Relaxation dynamics of the Kob-Andersen model (LJ units) by isothermal and equilibrium MD-DMS simulation at different temperatures. (a) Storage shear modulus  $G'$ , (b) loss shear modulus  $G''$ , (c) phase angle  $\delta$  and (d) IS  $D_{\min}$ .

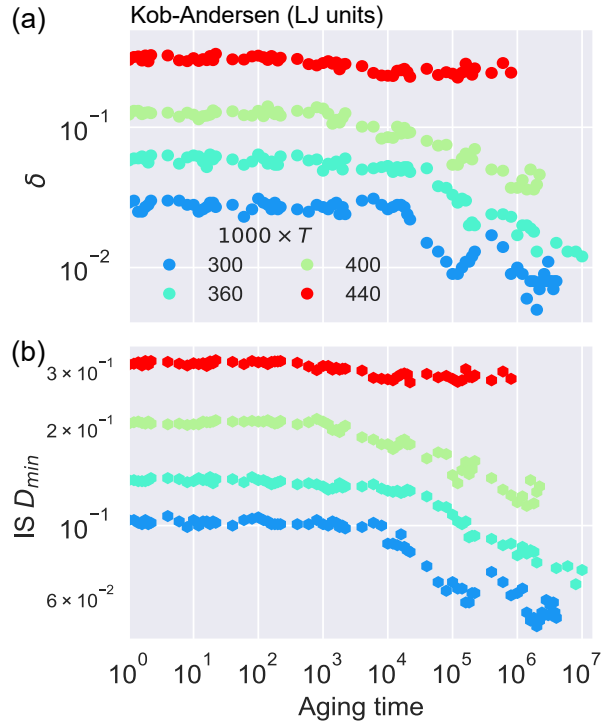

FIG. S5. (a) The phase angle  $\delta$  and (b) IS  $D_{\min}$  for Kob-Andersen model (LJ units) glass forming liquids as a function of aging at different temperatures as indicated.

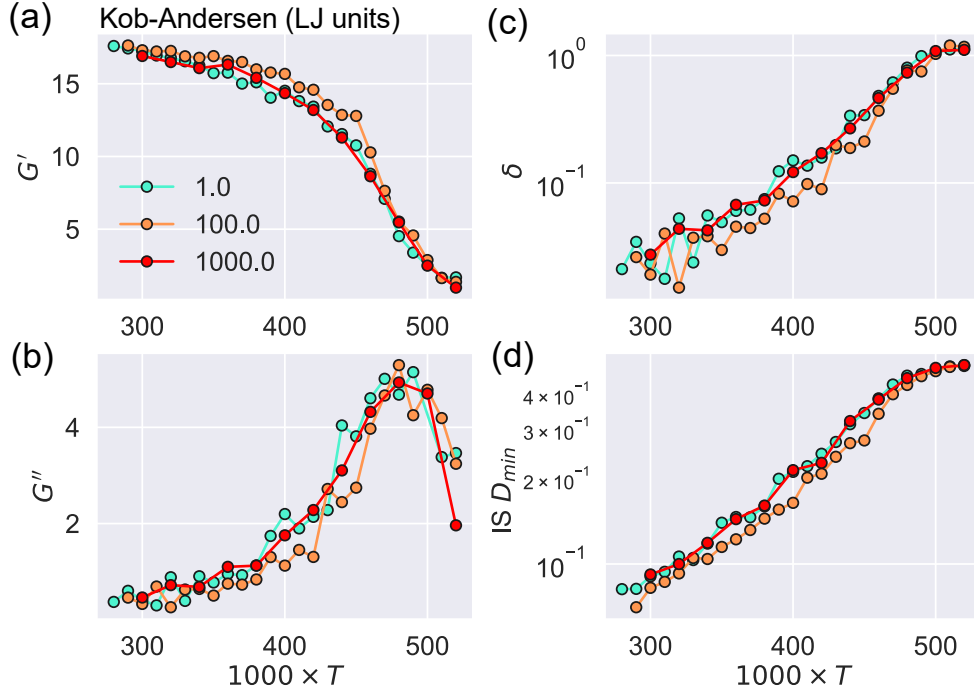

FIG. S6. Relaxation dynamics of the Kob-Andersen model (LJ units) obtained from MD-DMS simulations for different heating rates at a fixed cooling rate. (a) Storage shear modulus  $G'$ , (b) loss shear modulus  $G''$ , (c) phase angle  $\delta$  and (d) IS  $D_{\min}$ .

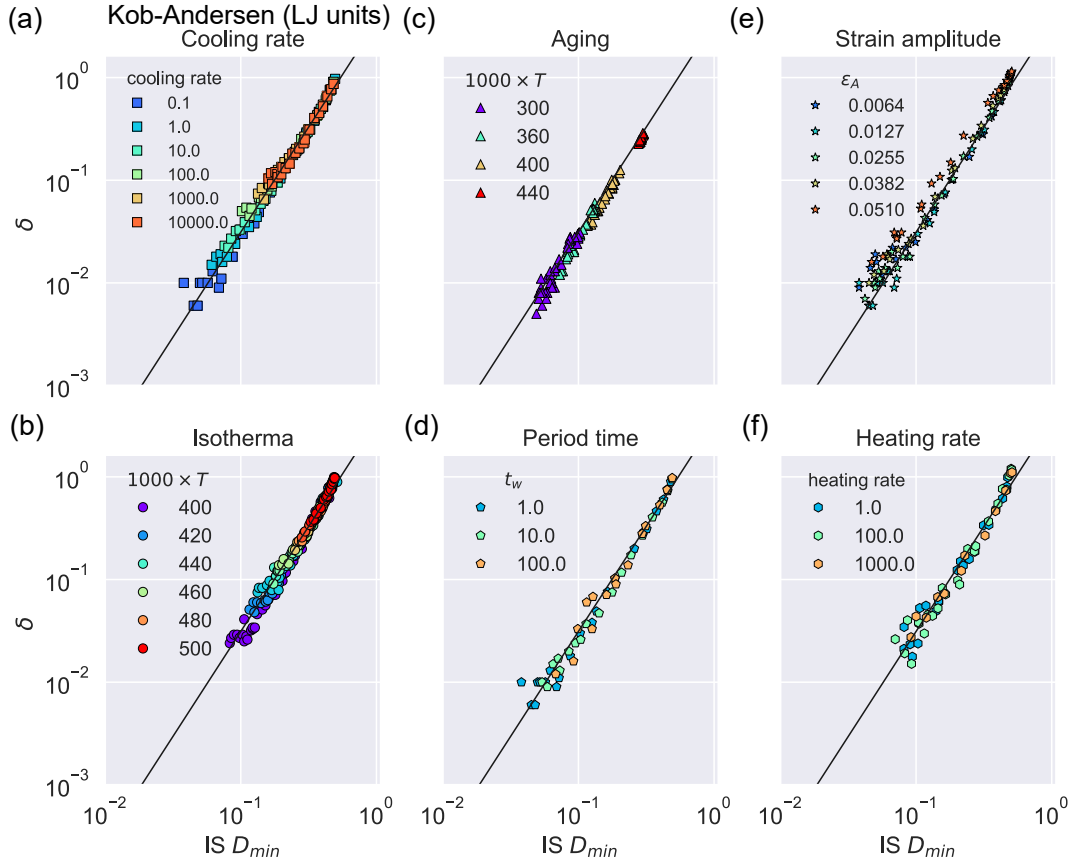

FIG. S7. Correlations of  $\delta$  and IS  $D_{\min}$  of the Kob-Andersen model (LJ units) at temperatures above  $T_0$  are obtained from MD-DMS at (a) cooling, (b) equilibrium, (c) aging, (d) oscillation period, (e) oscillation amplitude and (f) heating, respectively.

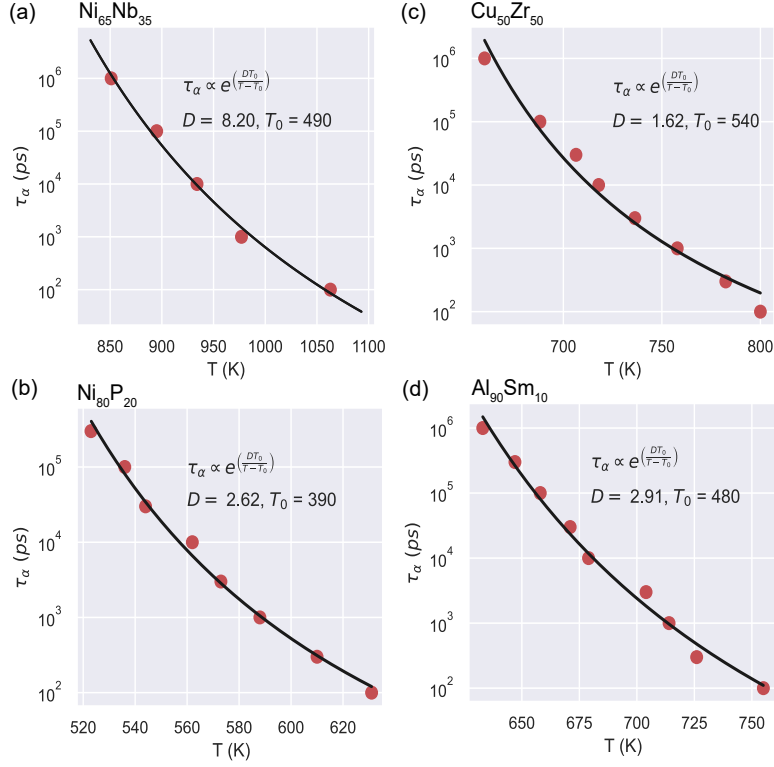

FIG. S8. The curve is fitted using the Vogel-Fulcher Tammann (VFT) equation  $\tau_\alpha = \tau_0 \exp(DT_0/T - T_0)$ , based on the peak times from isothermal and equilibrium MD-DMS measurements. The  $\alpha$ -relaxation time is determined to follow:  $\tau_\alpha \propto \exp(DT_0/T - T_0)$ , where  $D$  is the fragility parameter and  $T_0$  is the divergence temperature. The fitted parameters are: (a)  $\text{Ni}_{65}\text{Nb}_{35}$  ( $D = 8.20$ ,  $T_0 = 490$  K), (b)  $\text{Ni}_{80}\text{P}_{20}$  ( $D = 2.62$ ,  $T_0 = 390$  K), (c)  $\text{Cu}_{50}\text{Zr}_{50}$  ( $D = 1.62$ ,  $T_0 = 540$  K), and (d)  $\text{Al}_{90}\text{Sm}_{10}$  ( $D = 2.91$ ,  $T_0 = 480$  K).

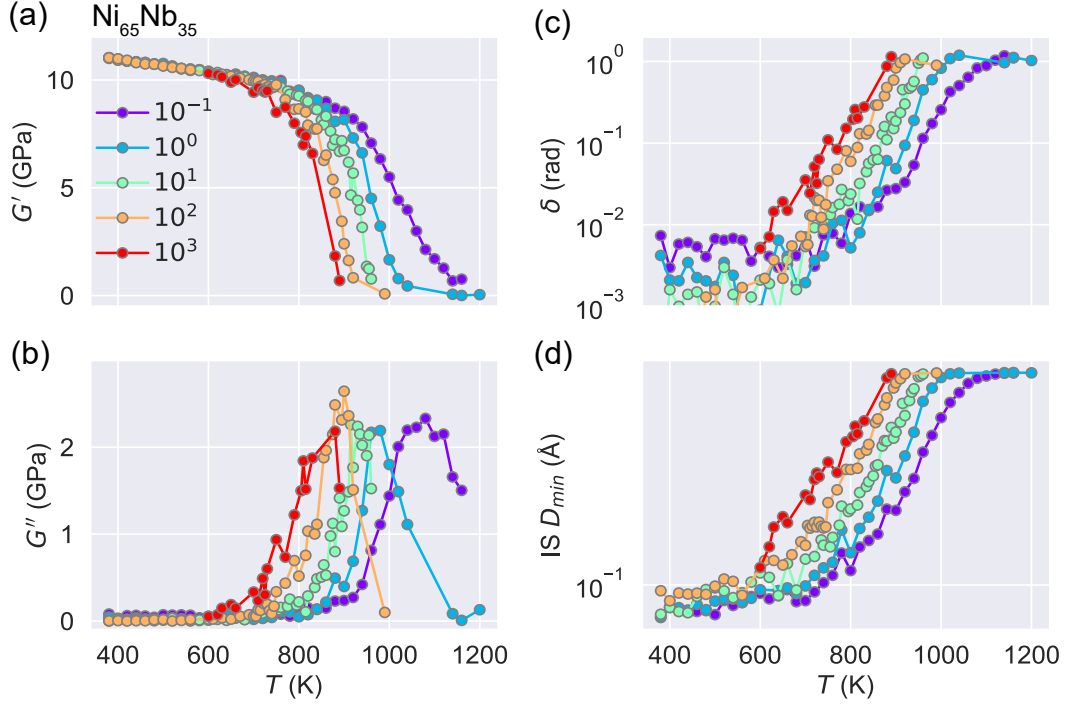

FIG. S9. Relaxation dynamics of the  $\text{Ni}_{65}\text{Nb}_{35}$  model by different  $t_\omega$  MD-DMS under the slowest cooling (0.1 K/ns). (a) Storage shear modulus  $G'$ , (b) loss shear modulus  $G''$ , (c) phase angle  $\delta$  and (d) IS  $D_{\min}$ .

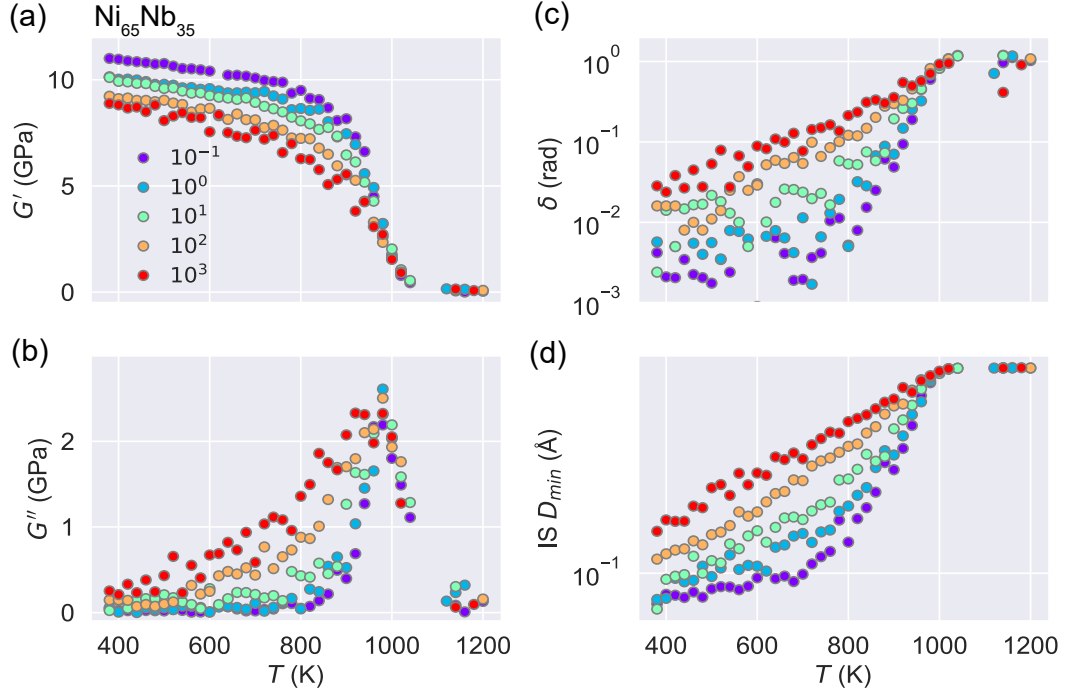

FIG. S10. Relaxation dynamics of the  $\text{Ni}_{65}\text{Nb}_{35}$  model obtained from MD-DMS simulations at 5 different cooling rates. (a) Storage shear modulus  $G'$ , (b) loss shear modulus  $G''$ , (c) phase angle  $\delta$  and (d) IS  $D_{\min}$ .

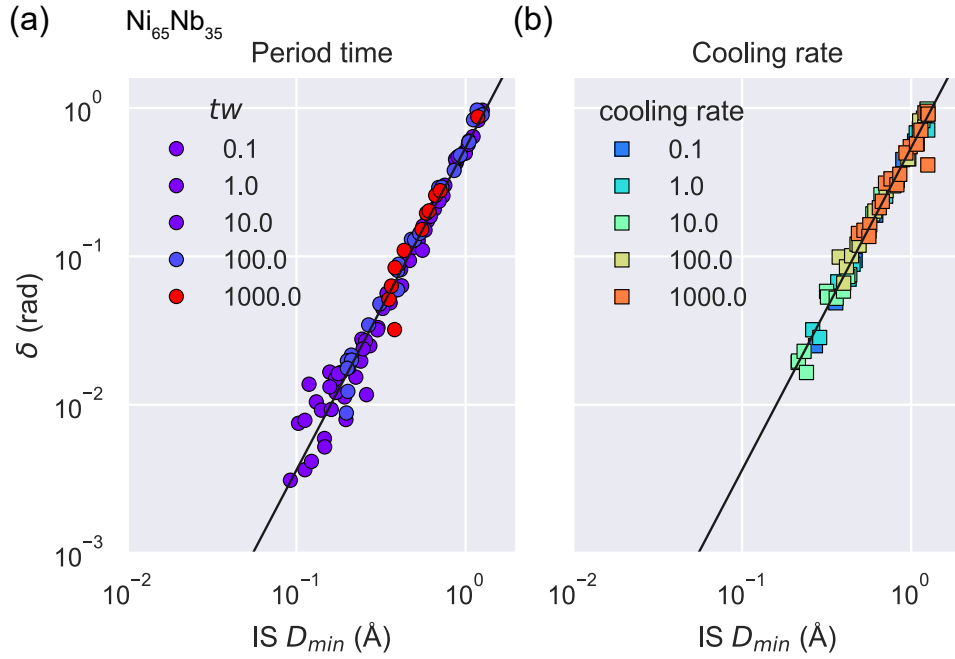

FIG. S11. Correlations of  $\delta$  and IS  $D_{\min}$  of the  $\text{Ni}_{65}\text{Nb}_{35}$  model at temperatures above  $T_0$  are obtained from MD-DMS at (a) periodic time (different periodic cycles at the slowest cooling rate), and (b) cooling rate.

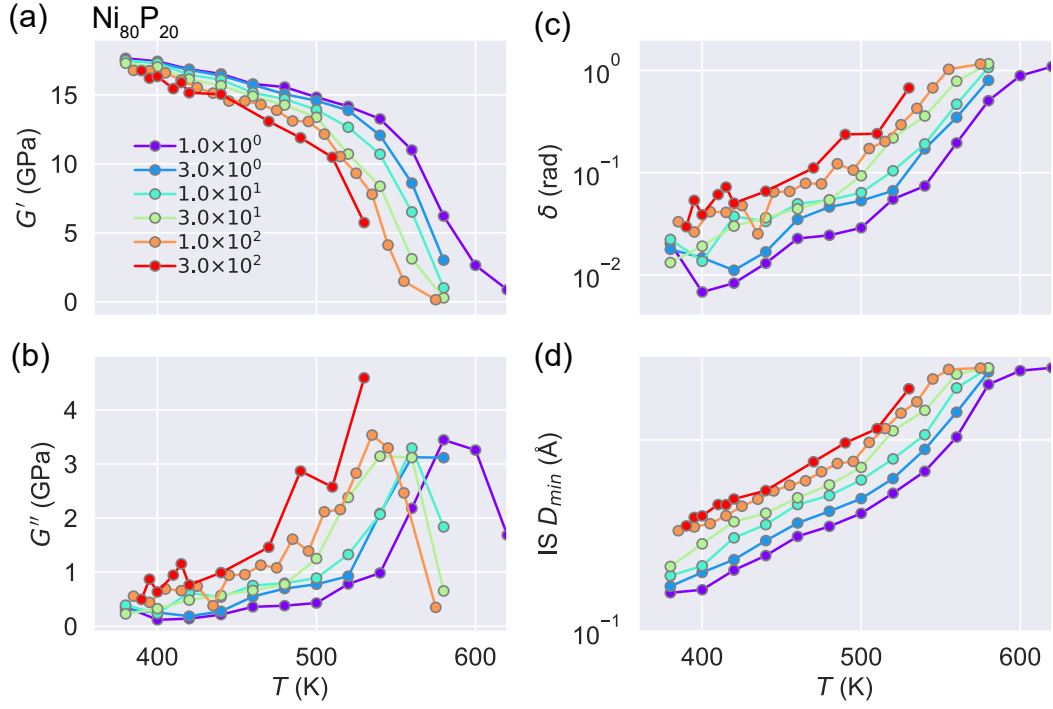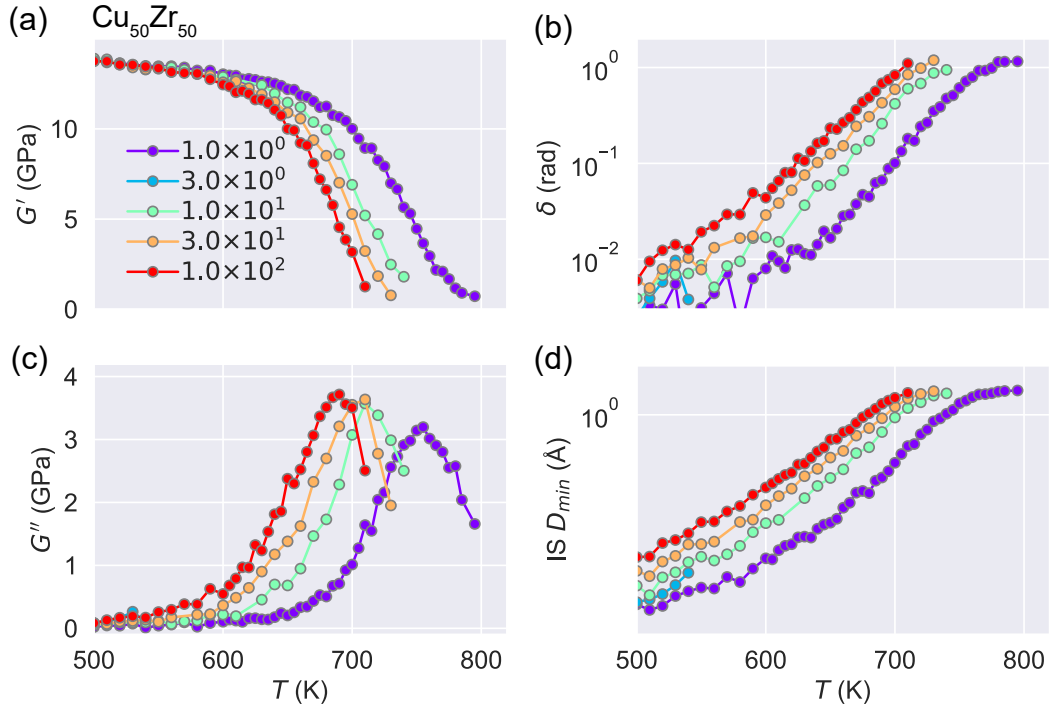



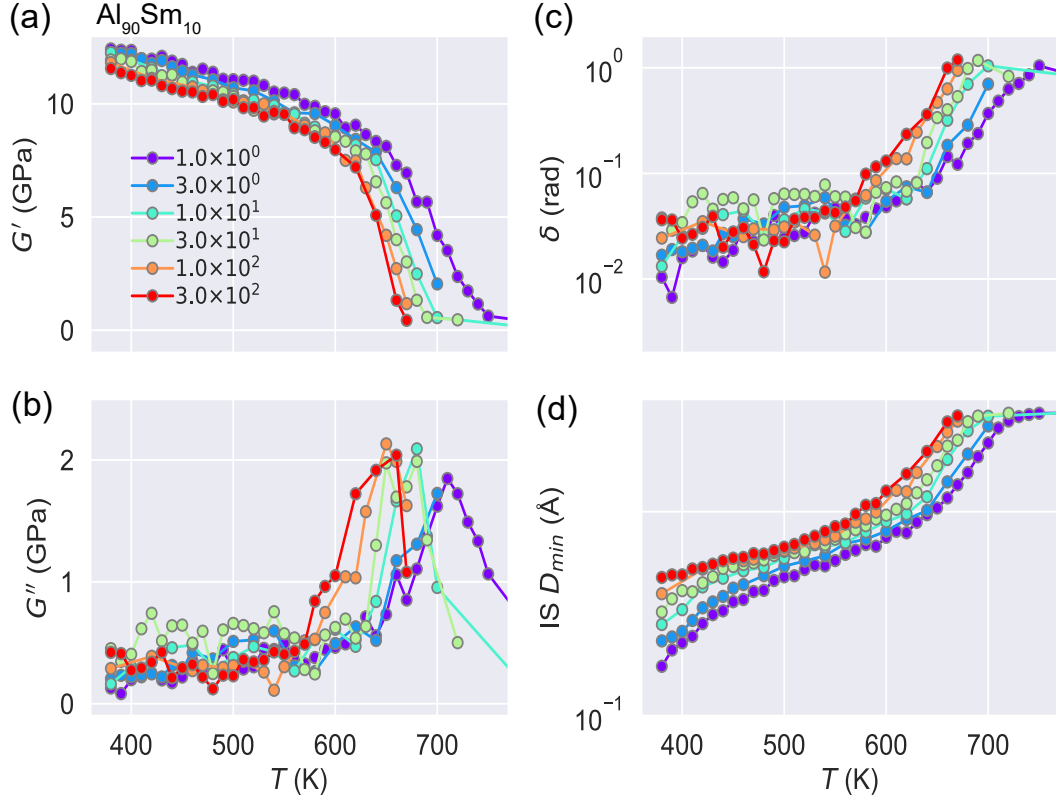

FIG. S14. Relaxation dynamics of the  $\text{Al}_{90}\text{Sm}_{10}$  model by different  $t_\omega$  MD-DMS under the same cooling rate. (a) Storage shear modulus  $G'$ , (b) loss shear modulus  $G''$ , (c) phase angle  $\delta$  and (d) IS  $D_{\min}$ .

- 
- [1] W. M. Brown and M. Yamada, Implementing molecular dynamics on hybrid high performance computers—three-body potentials, *Comput. Phys. Commun.* **184**, 2785 (2013).
  - [2] A. P. Thompson, H. M. Aktulga, R. Berger, D. S. Bolintineanu, W. M. Brown, P. S. Crozier, P. J. in 't Veld, A. Kohlmeyer, S. G. Moore, T. D. Nguyen, R. Shan, M. J. Stevens, J. Tranchida, C. Trott, and S. J. Plimpton, LAMMPS - a flexible simulation tool for particle-based materials modeling at the atomic, meso, and continuum scales, *Comput. Phys. Commun.* **271**, 108171 (2022).
  - [3] Y. Zhang, R. Ashcraft, M. Mendelev, C. Z. Wang, and K. F. Kelton, Experimental and molecular dynamics simulation study of structure of liquid and amorphous  $\text{Ni}_{62}\text{Nb}_{38}$  alloy, *J. Chem. Phys.* **145**, 204505 (2016).
  - [4] W. Kob and H. C. Andersen, Kinetic lattice-gas model of cage effects in high-density liquids and a test of mode-coupling theory of the ideal-glass transition, *Phys. Rev. E* **48**, 4364 (1993).
  - [5] L. Gao, H.-B. Yu, T. B. Schröder, and J. C. Dyre, Unified percolation scenario for the  $\alpha$  and  $\beta$  processes in simple glass formers, *Nat. Phys.* **21**, 471 (2025).
  - [6] K. Ngai, Universal properties of relaxation and diffusion in complex materials: Originating from fundamental physics with rich applications, *Prog. Mater. Sci.* **139**, 101130 (2023).
  - [7] L. Wang, N. Xu, W. H. Wang, and P. Guan, Revealing the link between structural relaxation and dynamic heterogeneity in glass-forming liquids, *Phys. Rev. Lett.* **120**, 125502 (2018).
  - [8] D. F. Crouse, On implementing 2D rectangular assignment algorithms, *IEEE Trans. Aerosp. Electron. Syst.* **52**, 1679 (2016).
